# Supplementary material for: Parametric Complexity Bounds for Approximating PDEs with Neural Networks
Source: arXiv:2103.02138 source file (2021-07-06)
Supplement: Supplementary file 1 [file additional_helper_lemmas.tex]

\section{Additional Helper Lemmas}
\begin{definition}[Angles between subspaces]
    \Tnote{TODO:Add definitions here}
\end{definition}
    
Assuming that $V = \Keigenfunctions$ and $\tilde{V} = \Keigenfunctionsapprox$ and 
$V_\perp = \spn\{\varphi_{k+1}, \ldots, \varphi_{\infty}\}$ 
and 
$V_\perp = \spn\{\tvarphi_{k+1}, \ldots, \tvarphi_{\infty}\}$
% $\tilde{V}_\perp = \spn\{\varphi_{k+1}, \ldots, \varphi_{\infty}\}$
We define 
$$
\cos \Theta(V, \hat{V}) 
= \inf_{\substack{x \in V, y \in \tilde{V} \\ \|x\|_{\l2} = 1 \\ \|y\|_{\l2} = 1}}
\langle x, y\rangle_{\l2}
$$
\Tnote{Cos here is defined with $\inf$ to match the $\sigma_{\min}$ in Andrej's paper definition.}
$$
\sin \Theta(V, \hat{V}) 
= \sup_{\substack{x \in V_\perp, y \in \tilde{V} \\ \|x\|_{\l2} = 1 \\ \|y\|_{\l2} = 1}}
\langle x, y\rangle_{\l2}
$$

\begin{align*}
    d_c(V, \tilde{V}) 
    &= \min_O\sup_{\substack{a \in \R^k \\ \sum_{i=1}^k a_i = 1}} \|\sum_{i=1}^k (O\varphi_i - \tvarphi_i)a_i\|_{\l2} \\
    &= \min_O \sup_{\substack{x \in V, y \in \tilde{V}\\ \|x\|_{\l2} = 1 \\ \|y\|_{\l2} = 1}} \|Oy - x\|_{\l2} \\
    &= \min_O \sup_{\substack{x \in V, y \in \tilde{V}\\ \|x\|_{\l2} = 1 \\ \|y\|_{\l2} = 1}} \sqrt{\|Oy - x\|^2_{\l2}} \\
    &= \min_O \sup_{\substack{x \in V, y \in \tilde{V}\\ \|x\|_{\l2} = 1 \\ \|y\|_{\l2} = 1}}
        \sqrt{\langle Oy, Oy\rangle_{\l2} + \langle x, x \rangle_{\l2} - 2\langle Oy, x \rangle_{\l2}}\\
    &= 2 \left( 1 - 
        \max_O \inf_{\substack{x \in V, y \in \tilde{V}\\ \|x\|_{\l2} = 1 \\ \|y\|_{\l2} = 1}} \sqrt{\langle Oy, x\rangle_{\l2}}
        \right) 
        \numberthis \label{eq:distance_final_form_but_one}
\end{align*}

Now, looking at the following term,
\begin{align*}
    \max_O \inf_{\substack{x \in V, y \in \tilde{V}\\ \|x\|_{\l2} = 1 \\ \|y\|_{\l2} = 1}} \langle Oy, x\rangle_{\l2}
    \geq \inf_{\substack{x \in V, y \in \tilde{V}\\ \|x\|_{\l2} = 1 \\ \|y\|_{\l2} = 1}} \langle y, x\rangle_{\l2}
    = \cos \Theta(V, \tilde{V})
    \numberthis \label{eq:max_cos_relation}
\end{align*}

Therefore from \eqref{eq:distance_final_form_but_one} and \eqref{eq:max_cos_relation} we have
\begin{align*}
    d_c(V, \tilde{V}) \leq \sqrt{2\left(1 - \cos\Theta(V, \tilde{V})\right)} = \|2\sin\frac{\Theta(V, \tilde{V})}{2}\|_2
\end{align*}

Further, we define $\sin \Theta(V, \tilde{V})$ as follows,
$$\sin \Theta(V, \tilde{V}) 
= 
\sup_{\substack{x \in V_\perp, y \in \tilde{V}\\ \|x\|_{\l2}\\ \|y\|_{\l2}}}\langle x, y\rangle_{\l2}$$
